# Supplementary material for: On the Elasticity of Polymer Model Networks Containing Finite Loops
Source: arXiv:2103.16181 source file (2021-03-30)
Supplement: Supplementary file 1 [file SI.pdf]

# On the elasticity of polymer model networks containing finite loops - Supporting information

Michael Lang*

*Leibniz Institute of Polymer Research Dresden, Hohe Stra?e 6, 01069 Dresden, Germany*

E-mail: lang@ipfdd.de

*To whom correspondence should be addressed

```fortran
Program recoursive
implicit none

integer max_i,max_f,i,f          ! i is loop size and f is functionality
Parameter (max_i = 10)           ! output is commented below
Parameter (max_f = 8)
double precision e,de
double precision DX,X,Nk(max_i,max_f)
double precision K,N,Ni,K2,K1,Kp,Km,Kk,Kav,Nx

N = 1.0
write(*,*) 'f, i, e(i,f), X(i,f), Delta_e(i,f)'

do f = 3,max_f
  i = 1
  K = N*DBLE(f-1)/DBLE(f-2)
  K2 = K/DBLE(f-2)
  Kp = 0.0
  Km = 0.0
  do i = 1,max_i
    if (i .eq. 1) then
      e = 0.0
      X = K2
      Nk(i,f) = 0.0
      K1 = K2
      Kk = K2
    else
      Nk(i,f) = Nk(i-1,f) + N + Nk(i-1,f)*N/Kk
      if (i .gt. 2) then
        Km = Nk(i-1,f) + Kk + Kk*Nk(i-1,f)/N
        Kp = N + Kk + Kk*N/Nk(i-1,f)
        K1 = K1*Km/(K1+Km)
        Kk = K2*Kp/(K2+Kp)
        Kav = (K1+Kk)/2.0
      else
        Kav = K2
      endif
      Ni = (2.0*Nk(i,f)*Kav)/(2.0*Kav+Nk(i,f))
      e = 1.0/(N+Ni)                   ! elastic "effectiveness" of a chain inside the loop
      Nx = Nk(i,f)*N/(Nk(i,f)+N)
      X = Kav*(Nx+Kav)/(Nx+2.0*Kav)    ! virtual strand for cross-link fluctuations
    endif                              ! inside the loop
    DX = X-K/DBLE(f)                   ! Delta X
    de = DBLE(f-2)/DBLE(f) - e + DX/K2 ! net change in elastic effectiveness
    write(*,*) f,i,e,X,DX,de
  enddo
enddo

end
```
